# Supplementary material for: Converging TDDFT calculations in 5 iterations with minimal auxiliary preconditioning
Source: arXiv:2404.17133 ancillary file (2024-04-26)
Supplement: Supplementary file 1 [file supplement.pdf]

Supplementary Materials for

# Converging TDDFT calculations in 5 iterations with minimal auxiliary preconditioning

Zehao Zhou(周泽浩) and Shane M. Parker[a]
*Department of Chemistry, Case Western Reserve University*
*10900 Euclid Ave, Cleveland, OH 44106, USA*

## I. MOLECULE TEST SETS

### A. TUNE8

The TUNE8 set was used to tune the $\theta$ parameter of the rid preconditioner. The molecules contained in TUNE8 are collected in Table SI.

TABLE SI: Molecules in TUNE8 set, $N_{at}$ is the number of atoms and $N_{bf}$ is the number of basis functions using def2-SVP basis set.

| No. | Molecules | $N_{at}$ | $N_{bf}$ |
|---|---|---|---|
| 1 | Si nanoparticle[1] | 21 | 218 |
| 2 | firefly luciferin | 26 | 300 |
| 3 | coumarin 153 | 36 | 378 |
| 4 | DAPI[2] | 36 | 369 |
| 5 | fluorescein | 37 | 410 |
| 6 | Rpet[3] | 37 | 404 |
| 7 | PyrImid TMIO5[4] | 43 | 413 |
| 8 | retinal | 49 | 434 |

### B. PRECOND19

The PRECOND19 set was used to benchmark the performance of the rid preconditioner. The molecules contained in PRECOND19 are collected in Table SII.

[a]Electronic mail: shane.parker@case.edu

TABLE SII: Molecules in PRECOND19 set, $N_{at}$ is the number of atoms and $N_{bf}$ is the number of basis functions using def2-TZVP basis set.

| No. | Molecules | $N_{at}$ | $N_{bf}$ |
|---|---|---|---|
| 1 | Si nanoparticle[1] | 21 | 399 |
| 2 | firefly luciferin | 26 | 618 |
| 3 | coumarin 153 | 36 | 766 |
| 4 | DAPI[2] | 36 | 741 |
| 5 | fluorescein | 37 | 847 |
| 6 | Rpet[3] | 37 | 815 |
| 7 | PyrImid TMIO5[4] | 43 | 808 |
| 8 | azobenzene 3a[5] | 46 | 1201 |
| 9 | DBF C5[6] | 47 | 932 |
| 10 | retinal | 49 | 819 |
| 11 | triphenylamino 5[7] | 49 | 1050 |
| 12 | coelenterazine[8] | 53 | 1118 |
| 13 | DPP1[9] | 55 | 1278 |
| 14 | cypridina luciferin | 57 | 1092 |
| 15 | merocyanine | 70 | 1351 |
| 16 | provitamin D3 | 72 | 1132 |
| 17 | protoporphyrin | 76 | 1506 |
| 18 | dinoflagellate luciferin | 83 | 1573 |
| 19 | 1'-hydroxy-$\gamma$-carotene | 99 | 1619 |

## II. OPTIMIZING INITIAL GUESS STRATEGY

The number of initial vectors used in the Davidson algorithm can significantly influence the efficiency of the algorithm. Adding additional initial guesses almost always decreases $N_{\text{iter}}$ by improving the description of the eigenvector in the first iteration. On the other hand, additional initial vectors can help or hurt $N_{\text{mv}}$, depending on the quality of the approximate eigenvector in the first iteration. Therefore, we revisited the performance of the rid preconditioner for TDA excitation energies by computing 10 states, using PBE0/def2-TZVP[10,11] for different numbers of extra initial vectors, $N_{\text{ex}}$. The number if initial vectors is chosen to be $N_{\text{init}} = \min(2N_{\text{states}}, N_{\text{states}} + N_{\text{ex}})$. The results are shown in Fig. S1. Overall, we find that the more effective the preconditioner, the fewer additional initial guesses should be included to minimize $N_{\text{mv}}$. Including up to 3 extra initial guess vectors for the rid preconditioner minimizes $N_{\text{iter}}$ but has minimal influence on $N_{\text{mv}}$. By contrast, for both diagonal and sTDA preconditioners, we find that adding up to 8 additional guesses reduces $N_{\text{iter}}$, and can even reduce $N_{\text{mv}}$. These results suggest that the initial guesses produced by the rid approximation are excellent starting vectors for the Davidson algorithm.

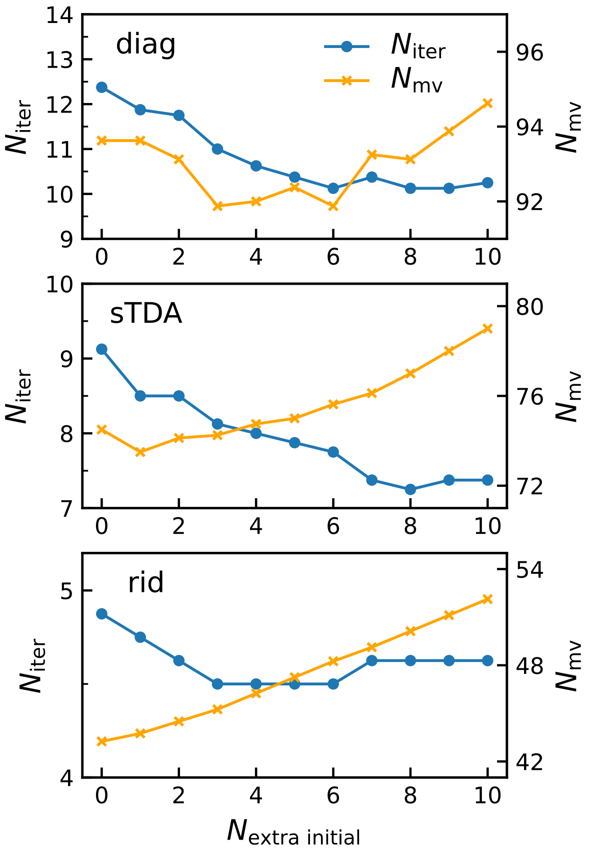


FIG. S1: The average number of iterations and matrix-vector products for the TUNE8 set, using diag, sTDA, and rid preconditioners with different number of additional initial guesses. 10 TDA excitation energies were computed using PBE0/def2-TZVP.

## III. PERFORMANCE OF THE RID PRECONDITIONER: TDDFT

In this section, the performance of the rid preconditioner is evaluated for computing eigenvalues of the TDDFT equations (i.e., without the Tamm–Dancoff approximation[12]). The data are collected in Fig. S2 and Table SIII. In all cases, the def2-TZVP basis set was used.

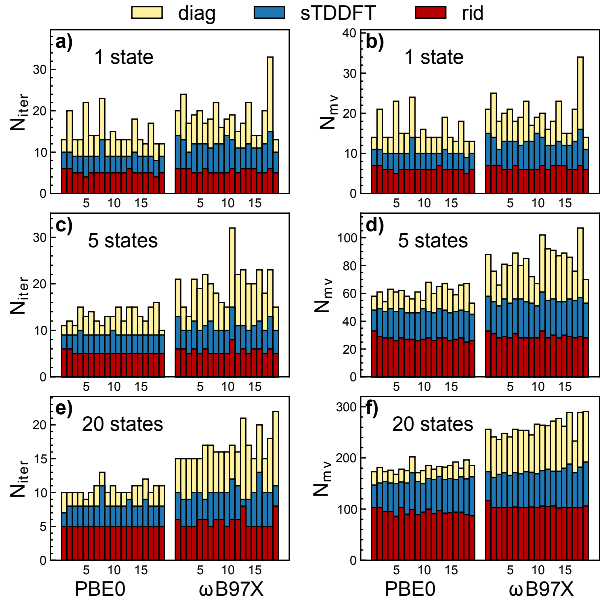


FIG. S2: Performance of the diagonal, sTDDFT, and rid preconditioners for computing TDDFT excitation energies. Left three panels show the number of iterations ($N_{\text{iter}}$), while the right three panels show the matrix-vector products ($N_{\text{mv}}$) required to converge 1, 5 or 20 states.

TABLE SIII: The range and the average number of iterations, $N_{\text{iter}}$, required to compute TDDFT excitation energies using the PBE0 and $\omega$B97X density functionals with diagonal, sTDA and rid preconditioners.

| | | PBE0 | | | $\omega$B97X | | |
|---|---|---|---|---|---|---|---|
| | preconditioner | diag | sTDA | rid | diag | sTDA | rid |
| $N_{\text{iter}}$ | range | 9–23 | 7–13 | 4–6 | 13–33 | 9–15 | 5–8 |
| | avg. 12.8 | 8.9 | 5.1 | 18.5 | 11.1 | 5.6 | |
| $\zeta_{\text{iter}}$ | range | – | 1.1–2.4 | 1.8–5.5 | – | 1.3–2.3 | 2.3–5.5 |
| | avg. | – | 1.4 | 2.6 | – | 1.7 | 3.3 |

## IV. COMPLETE BENCHMARK DATA

The complete benchmark data for the TDA, TDDFT, static and dynamic polarizability calculations are provided in the following tables.

TABLE SIV: $N_{\text{iter}}$ and $N_{\text{mv}}$ for TDA-TDDFT/PBE0/def2-TZVP excitation energy calculations, with different preconditioners.

| | $N_{\text{iter}}$ | | | | | | | | | $N_{\text{mv}}$ | | | | | | | | |
|---|---|---|---|---|---|---|---|---|---|---|---|---|---|---|---|---|---|---|
| states | 1 state | | | 5 states | | | 20 states | | | 1 state | | | 5 states | | | 20 states | | |
| Molecules Preconditioner | diag | sTDA | rid | diag | sTDA | rid | diag | sTDA | rid | diag | sTDA | rid | diag | sTDA | rid | diag | sTDA | rid |
| Si nanoparticle | 12 | 9 | 5 | 10 | 8 | 5 | 9 | 7 | 5 | 13 | 10 | 6 | 52 | 43 | 28 | 167 | 131 | 102 |
| firefly luciferin | 21 | 10 | 5 | 11 | 8 | 5 | 9 | 7 | 5 | 22 | 11 | 6 | 56 | 42 | 26 | 167 | 133 | 87 |
| coumarin 153 | 12 | 8 | 5 | 9 | 7 | 4 | 9 | 8 | 5 | 13 | 9 | 6 | 48 | 39 | 23 | 164 | 137 | 85 |
| DAPI | 11 | 8 | 4 | 12 | 9 | 5 | 9 | 7 | 4 | 12 | 9 | 5 | 55 | 43 | 24 | 162 | 137 | 83 |
| fluorescein | 19 | 7 | 4 | 12 | 8 | 4 | 9 | 7 | 4 | 20 | 8 | 5 | 54 | 41 | 23 | 154 | 132 | 82 |
| Rpet | 14 | 9 | 5 | 13 | 8 | 5 | 9 | 7 | 6 | 15 | 10 | 6 | 55 | 42 | 26 | 164 | 135 | 86 |
| PyrImid TMIO5 | 12 | 8 | 4 | 10 | 8 | 4 | 10 | 7 | 4 | 13 | 9 | 5 | 48 | 41 | 23 | 158 | 137 | 83 |
| azobenzene 3a | 20 | 11 | 5 | 10 | 8 | 4 | 12 | 11 | 5 | 21 | 12 | 6 | 49 | 40 | 23 | 184 | 151 | 86 |
| DBF C5 | 11 | 8 | 4 | 12 | 8 | 4 | 9 | 7 | 5 | 12 | 9 | 5 | 53 | 41 | 23 | 157 | 135 | 84 |
| retinal | 17 | 8 | 4 | 9 | 8 | 4 | 10 | 7 | 5 | 18 | 9 | 5 | 46 | 40 | 23 | 162 | 139 | 84 |
| triphenylamino 5 | 11 | 7 | 4 | 14 | 8 | 5 | 9 | 7 | 5 | 12 | 8 | 5 | 60 | 41 | 24 | 169 | 138 | 85 |
| coelenterazine | 12 | 8 | 4 | 11 | 7 | 4 | 9 | 7 | 4 | 13 | 9 | 5 | 54 | 39 | 23 | 162 | 140 | 83 |
| DPP1 | 11 | 8 | 4 | 13 | 8 | 5 | 10 | 8 | 5 | 12 | 9 | 5 | 59 | 41 | 24 | 169 | 144 | 87 |
| cypridina luciferin | 17 | 9 | 5 | 14 | 9 | 4 | 11 | 10 | 5 | 18 | 10 | 6 | 60 | 43 | 23 | 165 | 140 | 84 |
| merocyanine | 12 | 8 | 4 | 11 | 8 | 4 | 11 | 9 | 4 | 13 | 9 | 5 | 54 | 40 | 23 | 168 | 141 | 83 |
| provitamin D3 | 11 | 8 | 4 | 10 | 8 | 5 | 11 | 9 | 5 | 12 | 9 | 5 | 52 | 41 | 24 | 177 | 142 | 85 |
| protoporphyrin | 15 | 7 | 4 | 12 | 8 | 4 | 10 | 7 | 4 | 16 | 8 | 5 | 56 | 42 | 23 | 166 | 137 | 83 |
| dinoflagellate luciferin | 10 | 7 | 4 | 14 | 8 | 4 | 11 | 9 | 5 | 11 | 8 | 5 | 59 | 42 | 23 | 176 | 141 | 82 |
| 1'-hydroxy-$\gamma$-carotene | 11 | 8 | 4 | 9 | 8 | 4 | 10 | 8 | 5 | 12 | 9 | 5 | 46 | 40 | 23 | 167 | 142 | 84 |

TABLE SV: $N_{\text{iter}}$ and $N_{\text{mv}}$ for TDA-TDDFT/$\omega$B97X/def2-TZVP excitation energy calculations, with different preconditioners.

| | $N_{\text{iter}}$ | | | | | | | | | $N_{\text{mv}}$ | | | | | | | | |
|---|---|---|---|---|---|---|---|---|---|---|---|---|---|---|---|---|---|---|
| states | 1 state | | | 5 states | | | 20 states | | | 1 state | | | 5 states | | | 20 states | | |
| Molecules Preconditioner | diag | sTDA | rid | diag | sTDA | rid | diag | sTDA | rid | diag | sTDA | rid | diag | sTDA | rid | diag | sTDA | rid |
| Si nanoparticle | 18 | 10 | 5 | 20 | 11 | 5 | 15 | 10 | 5 | 19 | 11 | 6 | 84 | 51 | 28 | 257 | 168 | 103 |
| firefly luciferin | 25 | 12 | 6 | 15 | 9 | 5 | 14 | 8 | 5 | 26 | 13 | 7 | 73 | 47 | 28 | 236 | 156 | 100 |
| coumarin 153 | 15 | 9 | 5 | 12 | 8 | 5 | 16 | 10 | 5 | 16 | 10 | 6 | 60 | 43 | 26 | 234 | 156 | 90 |
| DAPI | 16 | 10 | 5 | 20 | 11 | 5 | 16 | 12 | 5 | 17 | 11 | 6 | 76 | 50 | 26 | 250 | 161 | 99 |
| fluorescein | 20 | 12 | 5 | 18 | 9 | 5 | 15 | 9 | 5 | 21 | 13 | 6 | 73 | 45 | 27 | 233 | 150 | 90 |
| Rpet | 15 | 10 | 5 | 21 | 11 | 5 | 16 | 9 | 5 | 16 | 11 | 6 | 83 | 49 | 28 | 246 | 155 | 100 |
| PyrImid TMIO5 | 16 | 9 | 5 | 17 | 12 | 5 | 16 | 9 | 5 | 17 | 10 | 6 | 71 | 50 | 25 | 244 | 157 | 91 |
| azobenzene 3a | 21 | 10 | 5 | 17 | 8 | 5 | 16 | 9 | 6 | 22 | 11 | 6 | 78 | 44 | 26 | 244 | 156 | 93 |
| DBF C5 | 14 | 9 | 5 | 14 | 8 | 5 | 17 | 9 | 5 | 15 | 10 | 6 | 64 | 45 | 24 | 237 | 156 | 90 |
| retinal | 18 | 13 | 5 | 16 | 9 | 5 | 16 | 9 | 5 | 19 | 14 | 6 | 64 | 44 | 26 | 258 | 158 | 93 |
| triphenylamino 5 | 17 | 10 | 5 | 33 | 10 | 9 | 16 | 13 | 7 | 18 | 11 | 6 | 96 | 48 | 31 | 255 | 165 | 97 |
| coelenterazine | 13 | 9 | 5 | 20 | 10 | 5 | 15 | 9 | 5 | 14 | 10 | 6 | 81 | 46 | 26 | 249 | 158 | 90 |
| DPP1 | 15 | 9 | 5 | 22 | 9 | 5 | 20 | 9 | 5 | 16 | 10 | 6 | 85 | 47 | 27 | 259 | 156 | 97 |
| cypridina luciferin | 22 | 10 | 5 | 18 | 9 | 5 | 16 | 9 | 5 | 23 | 11 | 6 | 82 | 47 | 27 | 253 | 157 | 93 |
| merocyanine | 12 | 9 | 5 | 18 | 10 | 5 | 15 | 10 | 5 | 13 | 10 | 6 | 82 | 47 | 26 | 245 | 159 | 93 |
| provitamin D3 | 13 | 9 | 5 | 21 | 10 | 5 | 19 | 13 | 5 | 14 | 10 | 6 | 79 | 48 | 28 | 282 | 179 | 95 |
| protoporphyrin | 17 | 9 | 4 | 20 | 10 | 5 | 14 | 11 | 5 | 18 | 10 | 5 | 74 | 47 | 24 | 218 | 153 | 84 |
| dinoflagellate luciferin | 30 | 14 | 6 | 19 | 9 | 5 | 17 | 9 | 5 | 31 | 15 | 7 | 88 | 46 | 25 | 277 | 165 | 92 |
| 1'-hydroxy-$\gamma$-carotene | 11 | 8 | 4 | 13 | 10 | 5 | 21 | 12 | 7 | 12 | 9 | 5 | 60 | 46 | 24 | 280 | 178 | 93 |

TABLE SVI: $N_{\text{iter}}$ and $N_{\text{mv}}$ for TDDFT/PBE0/def2-TZVP excitation energy calculations, with different preconditioners.

| | $N_{\text{iter}}$ | | | | | | | | | $N_{\text{mv}}$ | | | | | | | | |
|---|---|---|---|---|---|---|---|---|---|---|---|---|---|---|---|---|---|---|
| states | 1 state | | | 5 states | | | 20 states | | | 1 state | | | 5 states | | | 20 states | | |
| Molecules Preconditioner | diag | sTDA | rid | diag | sTDA | rid | diag | sTDA | rid | diag | sTDA | rid | diag | sTDA | rid | diag | sTDA | rid |
| Si nanoparticle | 13 | 10 | 6 | 11 | 9 | 6 | 10 | 7 | 5 | 14 | 11 | 7 | 58 | 48 | 33 | 173 | 147 | 103 |
| firefly luciferin | 20 | 10 | 6 | 12 | 9 | 6 | 10 | 8 | 5 | 21 | 11 | 7 | 61 | 49 | 29 | 181 | 151 | 103 |
| coumarin 153 | 13 | 9 | 5 | 11 | 9 | 5 | 10 | 8 | 5 | 14 | 10 | 6 | 54 | 47 | 28 | 173 | 154 | 95 |
| DAPI | 13 | 9 | 5 | 15 | 10 | 5 | 10 | 8 | 5 | 14 | 10 | 6 | 63 | 49 | 28 | 176 | 151 | 95 |
| fluorescein | 22 | 9 | 4 | 13 | 9 | 5 | 9 | 8 | 5 | 23 | 10 | 5 | 61 | 47 | 26 | 168 | 150 | 86 |
| Rpet | 14 | 9 | 5 | 14 | 9 | 5 | 10 | 8 | 5 | 15 | 10 | 6 | 62 | 49 | 28 | 178 | 153 | 103 |
| PyrImid TMIO5 | 14 | 9 | 5 | 12 | 9 | 5 | 11 | 8 | 5 | 15 | 10 | 6 | 58 | 46 | 27 | 175 | 151 | 90 |
| azobenzene 3a | 23 | 13 | 5 | 11 | 9 | 5 | 13 | 11 | 5 | 24 | 14 | 6 | 56 | 46 | 27 | 202 | 171 | 99 |
| DBF C5 | 13 | 9 | 5 | 13 | 9 | 5 | 10 | 8 | 5 | 14 | 10 | 6 | 61 | 46 | 26 | 171 | 154 | 89 |
| retinal | 15 | 9 | 5 | 13 | 10 | 5 | 11 | 8 | 5 | 16 | 10 | 6 | 55 | 49 | 27 | 175 | 150 | 94 |
| triphenylamino 5 | 13 | 9 | 5 | 15 | 9 | 5 | 10 | 8 | 5 | 14 | 10 | 6 | 68 | 47 | 28 | 185 | 160 | 100 |
| coelenterazine | 13 | 9 | 5 | 12 | 9 | 5 | 10 | 8 | 5 | 14 | 10 | 6 | 60 | 46 | 26 | 178 | 158 | 91 |
| DPP1 | 13 | 9 | 6 | 15 | 9 | 5 | 10 | 9 | 5 | 14 | 10 | 7 | 65 | 49 | 28 | 183 | 164 | 97 |
| cypridina luciferin | 18 | 10 | 5 | 15 | 9 | 5 | 11 | 8 | 5 | 19 | 11 | 6 | 67 | 48 | 28 | 182 | 158 | 92 |
| merocyanine | 13 | 9 | 5 | 13 | 9 | 5 | 11 | 8 | 5 | 14 | 10 | 6 | 63 | 46 | 26 | 185 | 160 | 93 |
| provitamin D3 | 12 | 9 | 5 | 12 | 9 | 5 | 12 | 9 | 5 | 13 | 10 | 6 | 59 | 47 | 27 | 192 | 158 | 94 |
| protoporphyrin | 17 | 9 | 5 | 15 | 9 | 5 | 10 | 8 | 5 | 18 | 10 | 6 | 66 | 48 | 28 | 180 | 163 | 94 |
| dinoflagellate luciferin | 12 | 8 | 4 | 16 | 9 | 5 | 11 | 8 | 5 | 13 | 9 | 5 | 67 | 47 | 25 | 196 | 159 | 89 |
| 1'-hydroxy-$\gamma$-carotene | 12 | 9 | 5 | 10 | 9 | 5 | 11 | 8 | 5 | 13 | 10 | 6 | 53 | 45 | 26 | 185 | 163 | 87 |

TABLE SVII: $N_{\text{iter}}$ and $N_{\text{mv}}$ for TDDFT/$\omega$B97X/def2-TZVP excitation energy calculations, with different preconditioners.

| | $N_{\text{iter}}$ | | | | | | | | | $N_{\text{mv}}$ | | | | | | | | |
|---|---|---|---|---|---|---|---|---|---|---|---|---|---|---|---|---|---|---|
| states | 1 state | | | 5 states | | | 20 states | | | 1 state | | | 5 states | | | 20 states | | |
| Molecules Preconditioner | diag | sTDA | rid | diag | sTDA | rid | diag | sTDA | rid | diag | sTDA | rid | diag | sTDA | rid | diag | sTDA | rid |
| Si nanoparticle | 20 | 14 | 6 | 21 | 13 | 6 | 15 | 10 | 6 | 21 | 15 | 7 | 88 | 58 | 33 | 256 | 173 | 117 |
| firefly luciferin | 24 | 13 | 6 | 15 | 10 | 6 | 15 | 9 | 5 | 25 | 14 | 7 | 76 | 54 | 31 | 241 | 162 | 103 |
| coumarin 153 | 17 | 10 | 6 | 13 | 10 | 5 | 15 | 9 | 5 | 18 | 11 | 7 | 66 | 51 | 28 | 236 | 168 | 103 |
| DAPI | 19 | 12 | 5 | 21 | 12 | 6 | 15 | 10 | 5 | 20 | 13 | 6 | 81 | 56 | 29 | 248 | 171 | 103 |
| fluorescein | 20 | 12 | 5 | 19 | 10 | 5 | 15 | 10 | 6 | 21 | 13 | 6 | 80 | 53 | 28 | 241 | 166 | 103 |
| Rpet | 17 | 12 | 6 | 22 | 11 | 6 | 17 | 9 | 6 | 18 | 13 | 7 | 89 | 56 | 31 | 256 | 171 | 104 |
| PyrImid TMIO5 | 18 | 11 | 5 | 20 | 12 | 5 | 17 | 10 | 5 | 19 | 12 | 6 | 80 | 56 | 28 | 254 | 169 | 103 |
| azobenzene 3a | 22 | 12 | 5 | 18 | 10 | 5 | 16 | 10 | 6 | 23 | 13 | 6 | 85 | 54 | 28 | 254 | 173 | 103 |
| DBF C5 | 16 | 12 | 5 | 16 | 10 | 5 | 16 | 10 | 6 | 17 | 13 | 6 | 72 | 53 | 28 | 245 | 172 | 104 |
| retinal | 18 | 14 | 5 | 15 | 10 | 5 | 16 | 10 | 5 | 19 | 15 | 6 | 67 | 51 | 28 | 266 | 169 | 103 |
| triphenylamino 5 | 19 | 13 | 6 | 32 | 15 | 8 | 17 | 12 | 6 | 20 | 14 | 7 | 102 | 61 | 33 | 264 | 175 | 106 |
| coelenterazine | 15 | 11 | 5 | 22 | 11 | 5 | 16 | 11 | 6 | 16 | 12 | 6 | 92 | 55 | 28 | 263 | 178 | 105 |
| DPP1 | 17 | 11 | 6 | 23 | 11 | 6 | 21 | 9 | 8 | 18 | 12 | 7 | 91 | 56 | 30 | 272 | 174 | 106 |
| cypridina luciferin | 22 | 12 | 6 | 20 | 10 | 5 | 17 | 9 | 5 | 23 | 13 | 7 | 87 | 54 | 28 | 277 | 174 | 102 |
| merocyanine | 14 | 11 | 6 | 20 | 11 | 6 | 15 | 10 | 5 | 15 | 12 | 7 | 89 | 54 | 30 | 262 | 180 | 103 |
| provitamin D3 | 14 | 11 | 5 | 23 | 12 | 6 | 20 | 13 | 5 | 15 | 12 | 6 | 86 | 56 | 29 | 289 | 188 | 103 |
| protoporphyrin | 20 | 12 | 5 | 18 | 10 | 5 | 15 | 10 | 5 | 21 | 13 | 6 | 76 | 55 | 28 | 233 | 171 | 103 |
| dinoflagellate luciferin | 33 | 15 | 6 | 23 | 13 | 6 | 18 | 10 | 5 | 34 | 16 | 7 | 107 | 57 | 29 | 289 | 182 | 103 |
| 1'-hydroxy-$\gamma$-carotene | 13 | 10 | 5 | 15 | 10 | 5 | 22 | 11 | 8 | 14 | 11 | 6 | 70 | 53 | 28 | 291 | 192 | 106 |

TABLE SVIII: $N_{\mathrm{iter}}$ and $N_{\mathrm{mv}}$ for polarizability calculations using PBE0 or $\omega$B97X, def2-TZVP, and the diag (d), sTDA (s), or rid (r) preconditioner.

| | static | | | | | | | | | | | | dynamic | | | | | | | | | | | |
|---|---|---|---|---|---|---|---|---|---|---|---|---|---|---|---|---|---|---|---|---|---|---|---|---|
| | PBE0 | | | | | | $\omega$B97X | | | | | | PBE0 | | | | | | $\omega$B97X | | | | | |
| | $N_{\mathrm{iter}}$ | | | $N_{\mathrm{mv}}$ | | | $N_{\mathrm{iter}}$ | | | $N_{\mathrm{mv}}$ | | | $N_{\mathrm{iter}}$ | | | $N_{\mathrm{mv}}$ | | | $N_{\mathrm{iter}}$ | | | $N_{\mathrm{mv}}$ | | |
| Molecules Preconditioner | d | s | r | d | s | r | d | s | r | d | s | r | d | s | r | d | s | r | d | s | r | d | s | r |
| Si nanoparticle | 9 | 10 | 6 | 27 | 29 | 18 | 11 | 10 | 6 | 33 | 30 | 18 | 10 | 10 | 6 | 30 | 30 | 18 | 11 | 10 | 6 | 33 | 30 | 18 |
| firefly luciferin | 12 | 10 | 6 | 34 | 30 | 18 | 13 | 11 | 6 | 38 | 33 | 18 | 12 | 11 | 6 | 35 | 31 | 18 | 14 | 12 | 6 | 39 | 34 | 18 |
| coumarin 153 | 11 | 10 | 6 | 32 | 29 | 17 | 13 | 11 | 6 | 37 | 32 | 18 | 12 | 10 | 6 | 34 | 29 | 17 | 14 | 11 | 6 | 40 | 32 | 18 |
| DAPI | 11 | 10 | 5 | 33 | 30 | 15 | 13 | 11 | 6 | 38 | 33 | 17 | 12 | 10 | 6 | 35 | 30 | 17 | 14 | 11 | 6 | 40 | 33 | 17 |
| fluorescein | 12 | 11 | 6 | 35 | 31 | 16 | 14 | 12 | 6 | 40 | 34 | 18 | 12 | 11 | 6 | 36 | 32 | 17 | 15 | 12 | 6 | 43 | 35 | 18 |
| Rpet | 12 | 11 | 6 | 35 | 31 | 18 | 13 | 12 | 6 | 38 | 33 | 18 | 12 | 11 | 6 | 35 | 32 | 18 | 14 | 12 | 6 | 40 | 34 | 18 |
| PyrImid TMIO5 | 12 | 10 | 5 | 34 | 30 | 15 | 13 | 11 | 6 | 38 | 33 | 17 | 12 | 10 | 6 | 35 | 30 | 16 | 14 | 11 | 6 | 40 | 33 | 18 |
| azobenzene 3a | 12 | 10 | 6 | 36 | 30 | 18 | 14 | 12 | 6 | 40 | 34 | 18 | 13 | 10 | 6 | 38 | 30 | 18 | 15 | 12 | 6 | 43 | 35 | 18 |
| DBF C5 | 12 | 10 | 6 | 33 | 29 | 17 | 14 | 11 | 6 | 39 | 32 | 17 | 13 | 10 | 6 | 37 | 29 | 17 | 14 | 12 | 6 | 40 | 34 | 17 |
| retinal | 11 | 10 | 6 | 33 | 30 | 16 | 12 | 11 | 6 | 36 | 32 | 18 | 12 | 11 | 6 | 35 | 31 | 16 | 13 | 11 | 6 | 38 | 32 | 18 |
| triphenylamino 5 | 12 | 10 | 6 | 35 | 29 | 16 | 13 | 12 | 6 | 39 | 34 | 18 | 13 | 10 | 6 | 37 | 29 | 16 | 14 | 12 | 6 | 41 | 34 | 18 |
| coelenterazine | 12 | 11 | 6 | 35 | 31 | 17 | 14 | 12 | 6 | 41 | 36 | 18 | 13 | 11 | 6 | 38 | 33 | 17 | 15 | 12 | 6 | 44 | 36 | 18 |
| DPP1 | 13 | 11 | 7 | 36 | 32 | 18 | 15 | 12 | 7 | 41 | 35 | 19 | 15 | 12 | 7 | 40 | 33 | 18 | 16 | 12 | 7 | 44 | 35 | 19 |
| cypridina luciferin | 12 | 10 | 5 | 34 | 30 | 15 | 13 | 11 | 6 | 39 | 33 | 18 | 12 | 10 | 6 | 35 | 30 | 16 | 14 | 12 | 6 | 41 | 34 | 18 |
| merocyanine | 12 | 11 | 6 | 35 | 32 | 18 | 14 | 12 | 6 | 39 | 34 | 18 | 13 | 11 | 6 | 36 | 32 | 18 | 15 | 12 | 6 | 42 | 34 | 18 |
| provitamin D3 | 11 | 10 | 6 | 31 | 30 | 16 | 12 | 11 | 6 | 34 | 31 | 18 | 11 | 10 | 6 | 32 | 30 | 17 | 12 | 11 | 6 | 34 | 32 | 18 |
| protoporphyrin | 13 | 10 | 6 | 38 | 30 | 17 | 15 | 12 | 6 | 44 | 35 | 18 | 15 | 11 | 6 | 43 | 32 | 17 | 18 | 13 | 6 | 53 | 38 | 18 |
| dinoflagellate luciferin | 12 | 11 | 6 | 36 | 31 | 18 | 13 | 11 | 6 | 39 | 33 | 18 | 13 | 11 | 6 | 37 | 32 | 18 | 14 | 11 | 6 | 42 | 33 | 18 |
| 1’-hydroxy-$\gamma$-carotene | 13 | 10 | 6 | 36 | 30 | 17 | 13 | 12 | 6 | 38 | 34 | 18 | 14 | 11 | 6 | 39 | 31 | 17 | 14 | 13 | 6 | 41 | 36 | 18 |

[1] Y. Shu and B. G. Levine, "Communication: Non-radiative recombination via conical intersection at a semiconductor defect," J. Chem. Phys. **139**, 081102 (2013).
[2] J. Kapuscinski, "Dapi: A dna-specific fluorescent probe," Biotech. Histochem. **70**, 220–233 (1995).
[3] T. M. Clarke, K. C. Gordon, W. M. Kwok, D. L. Phillips, and D. L. Officer, "Tuning from $\pi$,$\pi$* to charge-transfer excited states in styryl-substituted terthiophenes: an ultrafast and steady-state emission study," J. Phys. Chem. A **110**, 7696–7702 (2006).
[4] B. A. Chalmers, S. Saha, T. Nguyen, J. McMurtrie, S. T. Sigurdsson, S. E. Bottle, and K.-S. Masters, "Tmio-pyrimid hybrids are profluorescent, site-directed spin labels for nucleic acids," Org. Lett. **16**, 5528–5531 (2014).
[5] J. Yoshino, N. Kano, and T. Kawashima, "Synthesis of the most intensely fluorescent azobenzene by utilizing the b-n interaction," Chem. Commun. , 559–561 (2007).
[6] X. S. Shang, D. Y. Li, N. T. Li, and P. N. Liu, "A concise synthesis of tunable fluorescent 1,3-dihydroisobenzofuran derivatives as new fluorophores," Dyes Pigm. **114**, 8–17 (2015).
[7] T. Tao, B. Ma, Y. Peng, X. Wang, W. Huang, and X. You, "Asymmetrical/symmetrical d-$\pi$-a/d-$\pi$-d thiazole-containing aromatic heterocyclic fluorescent compounds having the same triphenylamino chromophores," J. Org. Chem. **78**, 8669–8679 (2013).
[8] R. Nishihara, H. Suzuki, E. Hoshino, S. Suganuma, M. Sato, T. Saitoh, S. Nishiyama, N. Iwasawa, D. Citterio, and K. Suzuki, "Bioluminescent coelenterazine derivatives with imidazopyrazinone c-6 extended substitution," Chem. Commun. **51**, 391–394 (2015).
[9] J. Warnan, L. Favereau, Y. Pellegrin, E. Blart, D. Jacquemin, and F. Odobel, "A compact diketopyrrolopyrrole dye as efficient sensitizer in titanium dioxide dye-sensitized solar cells," J. Photochem. Photobiol. A **226**, 9–15 (2011).
[10] J. P. Perdew, M. Ernzerhof, and K. Burke, "Rationale for mixing exact exchange with density functional approximations," J. Chem. Phys. **105**, 9982–9985 (1996).
[11] F. Weigend and R. Ahlrichs, "Balanced basis sets of split valence, triple zeta valence and quadruple zeta valence quality for h to rn: Design and assessment of accuracy," Phys. Chem. Chem. Phys. **7**, 3297–3305 (2005).
[12] S. Hirata and M. Head-Gordon, "Time-dependent density functional theory within the Tamm–Dancoff approximation," Chem. Phys. Lett. **314**, 291–299 (1999).
